# Supplementary material for: Digger: Detecting Copyright Content Mis-usage in Large Language Model Training
Source: arXiv:2401.00676 source file (2024-01-01)
Supplement: Supplementary file 1 [file 8-appendix-b.tex]

\section{APPENDIX }
    \label{appendix:b}
